# Supplementary material for: Accelerating the Convergence of Auxiliary-Field Quantum Monte Carlo inSolids with Optimized Gaussian Basis Sets
Source: arXiv:2008.06609 ancillary file (2020-08-18)
Supplement: Supplementary file 1 [file supplement.pdf]

**Supplementary information for ‘Accelerating the Convergence of Auxiliary-Field  
Quantum Monte Carlo in Solids with Optimized Gaussian Basis Sets’**

Miguel A. Morales<sup>1</sup> and Fionn D. Malone<sup>1</sup>

*Lawrence Livermore National Laboratory, Livermore, California 94550,  
USA*

(Dated: 27 July 2020)

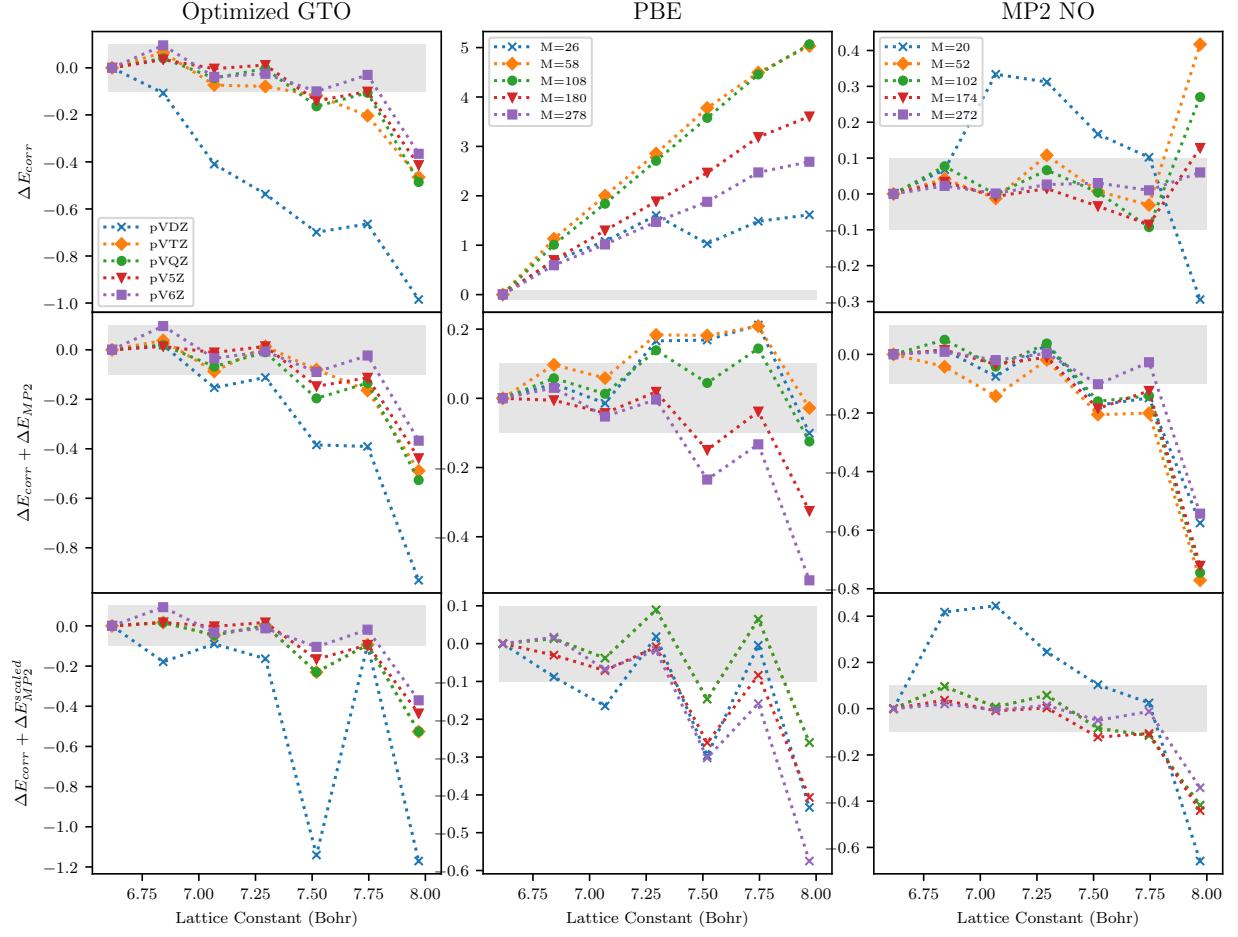

FIG. 1. LiH

## I. ADDITIONAL ERROR ANALYSIS OF COLD CURVES

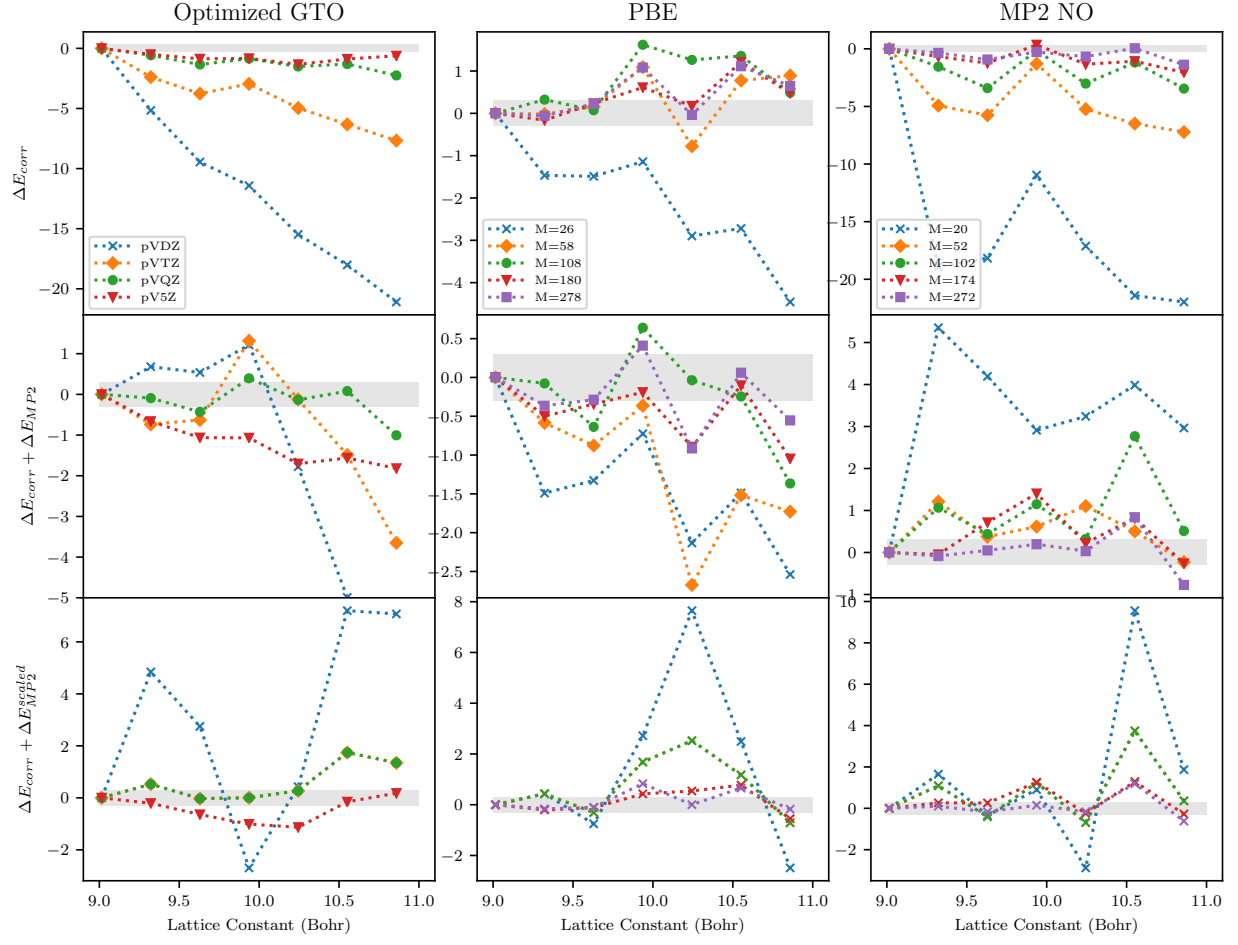

FIG. 2. Si
