# Supplementary material for: Accelerating the Convergence of Auxiliary-Field Quantum Monte Carlo inSolids with Optimized Gaussian Basis Sets
Source: arXiv:2008.06609 source file (2020-08-18)
Supplement: Supplementary file 2 [file supplement.pdf]

**Supplementary information for ‘Accelerating the Convergence of Auxiliary-Field  
Quantum Monte Carlo in Solids with Optimized Gaussian Basis Sets’**

Miguel A. Morales<sup>1</sup> and Fionn D. Malone<sup>1</sup>

*Lawrence Livermore National Laboratory, Livermore, California 94550,  
USA*

(Dated: 18 August 2020)

## I. COLD CURVES AND ERROR CANCELLATION

?? and ?? show a comparison of the non-parallelity errors in the correlation energy of Si and LiH. These figures show information equivalent to the results presented in the main manuscript for MgO. As discussed in the main text, the overall features in Si and LiH are consistent with those for MgO. PBE orbitals offer a good choice for Si, but they are quite poor for LiH. Both OPTM-GTO and MP2-NO orbitals are reasonable alternatives for LiH and Si. Scaled-MP2 basis set corrections offer a better performance over the bare correction in most cases.

## II. EQUATION OF STATE

Figures ??-?? show equation of state properties for MgO, LiH and Si for 2x2x2 and 3x3x3 *k-point* grids, corresponding to systems with 16 and 54 atoms in the unit cell. Results are shown for uncorrected AFQMC energies as well as energies with both bare and scaled MP2 corrections. In all cases, the scaling parameter in the scaled MP2 correction was calculated using pVTZ and pVQZ basis sets.

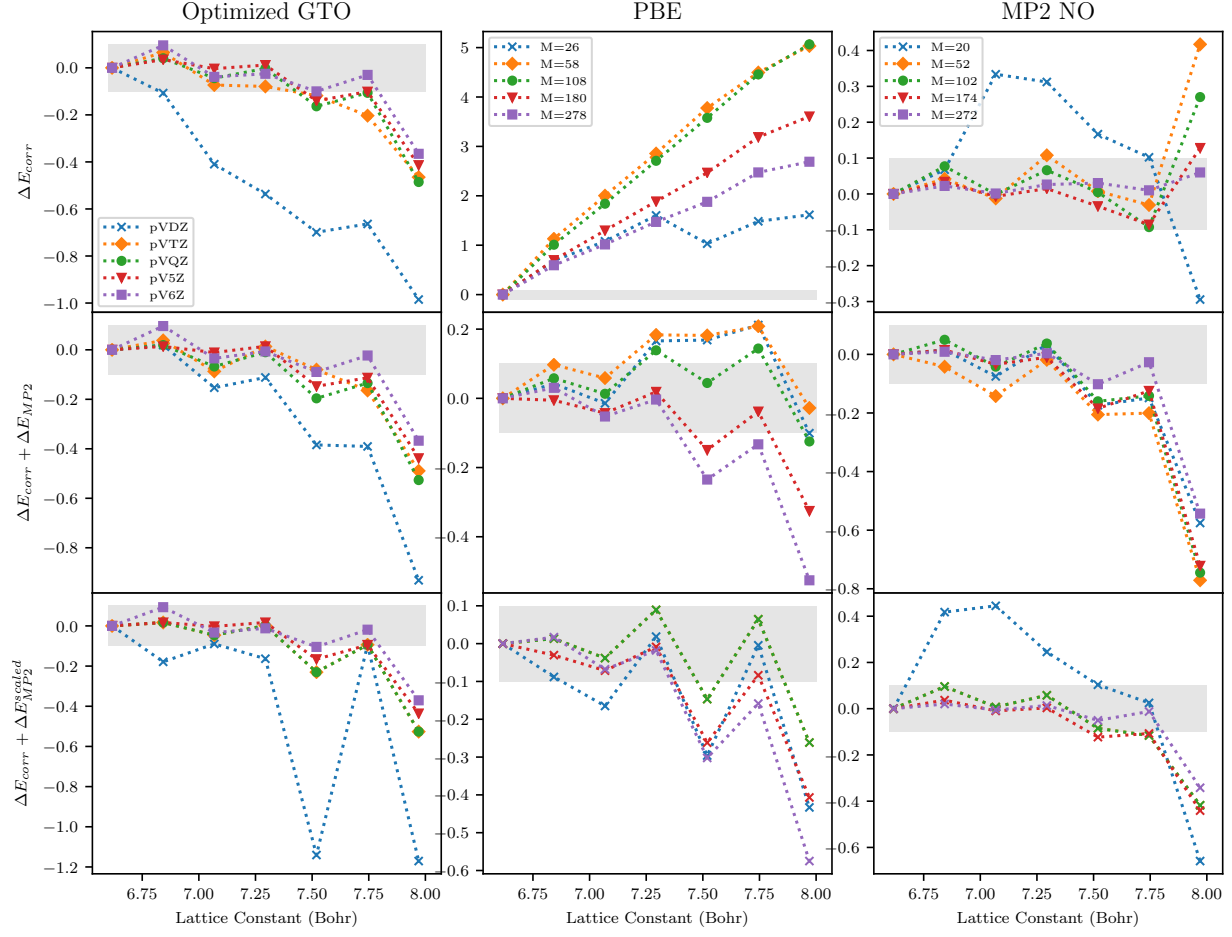

FIG. 1. Comparison between the calculated non-parallelity errors in the correlation energy ( $\Delta E(a)$ ) found in LiH for the three orbitals sets considered in this work (OPTM-GTO, PBE and MP2-NO). The first row shows the error in the uncorrected AFQMC correlation energy, while the middle and bottom rows show the reduction in error found when using either the standard MP2 correction ( $\Delta E_{\text{MP2}}$ ) or the scaled MP2 correction ( $\Delta E_{\text{MP2}}^{\text{scaled}}$ ) respectively. The shaded grey region represents the error in the CBS extrapolation.

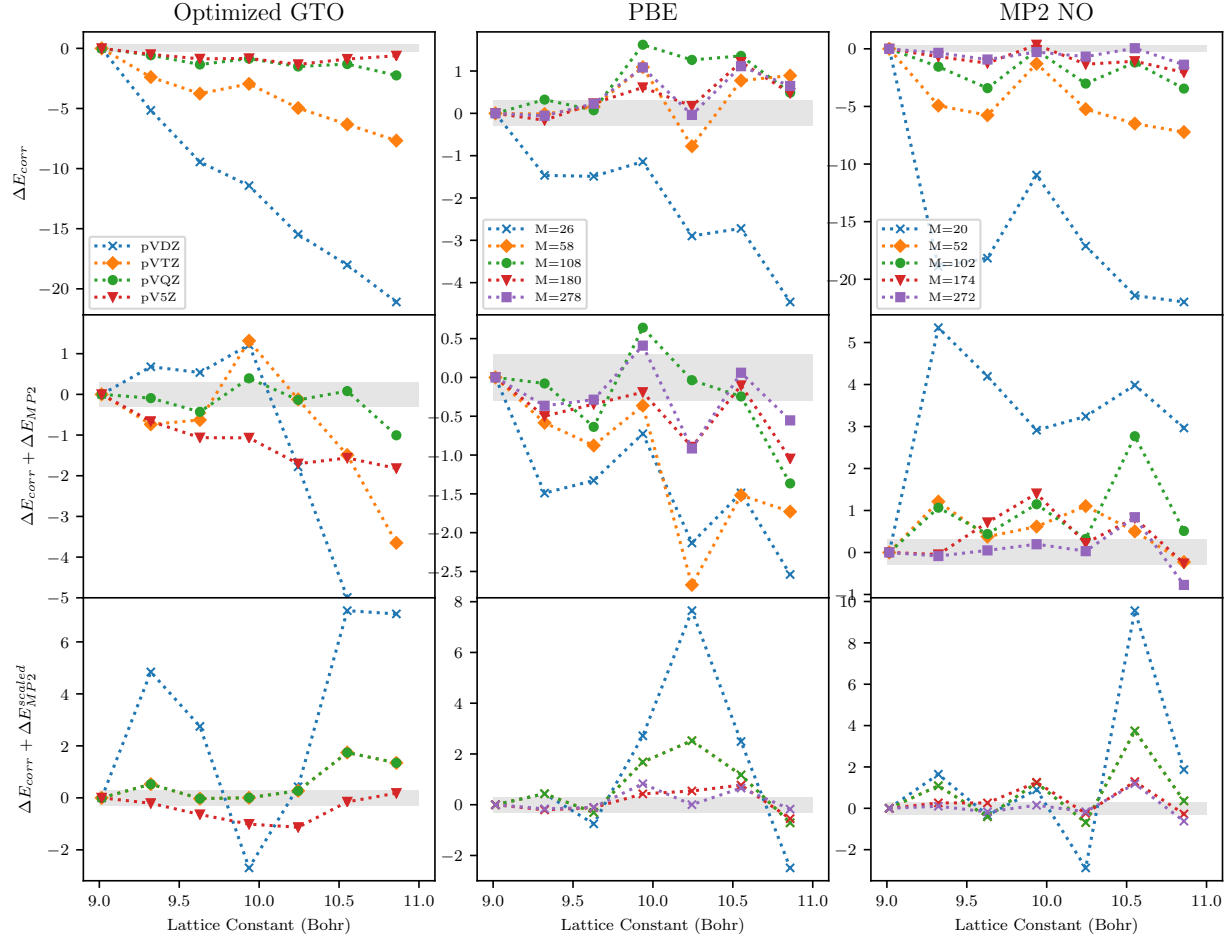

FIG. 2. Comparison between the calculated non-parallelity errors in the correlation energy ( $\Delta E(a)$ ) found in Si for the three orbitals sets considered in this work (OPTM-GTO, PBE and MP2-NO). The first row shows the error in the uncorrected AFQMC correlation energy, while the middle and bottom rows show the reduction in error found when using either the standard MP2 correction ( $\Delta E_{\text{MP2}}$ ) or the scaled MP2 correction ( $\Delta E_{\text{MP2}}^{\text{scaled}}$ ) respectively. The shaded grey region represents the error in the CBS extrapolation.

|                              | pVDZ     | pVTZ     | pVQZ     |
|------------------------------|----------|----------|----------|
| Lattice Constant (Bohr)      |          |          |          |
| Uncorrected                  | 7.931(2) | 7.914(3) | 7.892(3) |
| MP2 corrected                | 7.975(2) | 7.950(3) | 7.941(3) |
| Scaled MP2 corr.             | 7.929(2) | 7.928(3) | 7.929(3) |
| Bulk Modulus (GPa)           |          |          |          |
| Uncorrected                  | 188(2)   | 178(2)   | 183(3)   |
| MP2 corrected                | 143(2)   | 168(2)   | 166(3)   |
| Scaled MP2 corr.             | 144(2)   | 165(2)   | 166(3)   |
| Atomization Energy (eV/atom) |          |          |          |
| Uncorrected                  | 5.023(3) |          |          |
| MP2 corrected                | 5.386(3) | 5.361(3) | 5.311(3) |
| Scaled MP2 corr.             | 5.157(2) | 5.261(2) | 5.262(3) |

TABLE I. Lattice constant, bulk modulus and atomization energy of MgO calculated with a 3x3x3 *k-point* grid (corresponding to a 54 atom simulation cell), for various OPTM-GTO basis sets. Results with and without basis set corrections are presented.

|                              | pVDZ     | pVTZ     | pVQZ     |
|------------------------------|----------|----------|----------|
| Lattice Constant (Bohr)      |          |          |          |
| Uncorrected                  | 7.542(2) | 7.612(4) | 7.612(3) |
| MP2 corrected                | 7.617(2) | 7.609(3) | 7.612(3) |
| Scaled MP2 corr.             | 7.613(2) | 7.613(3) | 7.613(3) |
| Bulk Modulus (GPa)           |          |          |          |
| Uncorrected                  | 38.0(4)  | 32.6(9)  | 36.3(9)  |
| MP2 corrected                | 37.9(5)  | 37.5(9)  | 36.4(9)  |
| Scaled MP2 corr.             | 40.7(5)  | 36.5(9)  | 36.5(9)  |
| Atomization Energy (eV/atom) |          |          |          |
| Uncorrected                  | 2.414(1) |          |          |
| MP2 corrected                | 2.519(1) | 2.462(1) | 2.447(1) |
| Scaled MP2 corr.             | 2.409(1) | 2.442(1) | 2.442(1) |

TABLE II. Lattice constant, bulk modulus and atomization energy of LiH calculated with a 2x2x2 *k-point* grid for various OPTM-GTO basis sets. Results with and without basis set corrections are presented.

|                              | pVDZ     | pVTZ     | pVQZ     |
|------------------------------|----------|----------|----------|
| Lattice Constant (Bohr)      |          |          |          |
| Uncorrected                  | 7.420(2) | 7.556(3) | 7.560(3) |
| MP2 corrected                | 7.557(2) | 7.563(3) | 7.560(3) |
| Scaled MP2 corr.             | 7.504(2) | 7.558(3) | 7.559(3) |
| Bulk Modulus (GPa)           |          |          |          |
| Uncorrected                  | 43.0(3)  | 39.3(7)  | 38.8(8)  |
| MP2 corrected                | 37.6(5)  | 38.2(8)  | 38.7(8)  |
| Scaled MP2 corr.             | 37.8(4)  | 38.4(7)  | 38.4(8)  |
| Atomization Energy (eV/atom) |          |          |          |
| Uncorrected                  | 2.473(1) |          |          |
| MP2 corrected                | 2.543(1) | 2.514(1) | 2.502(1) |
| Scaled MP2 corr.             | 2.447(1) | 2.497(1) | 2.497(1) |

TABLE III. Lattice constant, bulk modulus and atomization energy of LiH calculated with a 3x3x3 *k-point* grid for various OPTM-GTO basis sets. Results with and without basis set corrections are presented.

|                              | pVDZ      | pVTZ      | pVQZ      |
|------------------------------|-----------|-----------|-----------|
| Lattice Constant (Bohr)      |           |           |           |
| Uncorrected                  | 10.323(2) | 10.272(2) | 10.257(2) |
| MP2 corrected                | 10.261(2) | 10.278(2) | 10.259(2) |
| Scaled MP2 corr.             | 10.189(2) | 10.247(2) | 10.247(2) |
| Bulk Modulus (GPa)           |           |           |           |
| Uncorrected                  | 96.0(8)   | 104.7(9)  | 105.5(9)  |
| MP2 corrected                | 99.3(7)   | 102.1(9)  | 103.8(9)  |
| Scaled MP2 corr.             | 104.7(6)  | 105.2(9)  | 105.2(9)  |
| Atomization Energy (eV/atom) |           |           |           |
| Uncorrected                  | 4.236(2)  |           |           |
| MP2 corrected                | 4.971(2)  | 4.757(2)  | 4.642(2)  |
| Scaled MP2 corr.             | 4.408(2)  | 4.569(2)  | 4.569(2)  |

TABLE IV. Lattice constant, bulk modulus and atomization energy of Si calculated with a 2x2x2 *k-point* grid for various OPTM-GTO basis sets. Results with and without basis set corrections are presented.



|                              | pVDZ      | pVTZ      | pVQZ      |
|------------------------------|-----------|-----------|-----------|
| Lattice Constant (Bohr)      |           |           |           |
| Uncorrected                  | 10.320(2) | 10.261(2) | 10.251(5) |
| MP2 corrected                | 10.274(2) | 10.267(2) | 10.260(5) |
| Scaled MP2 corr.             | 10.244(2) | 10.249(2) | 10.253(5) |
| Bulk Modulus (GPa)           |           |           |           |
| Uncorrected                  | 98(1)     | 101(1)    | 106(2)    |
| MP2 corrected                | 96.3(9)   | 99(1)     | 103(2)    |
| Scaled MP2 corr.             | 109.9(8)  | 103(1)    | 105(2)    |
| Atomization Energy (eV/atom) |           |           |           |
| Uncorrected                  | 4.438(3)  |           |           |
| MP2 corrected                | 5.046(20) | 4.926(3)  | 4.864(3)  |
| Scaled MP2 corr.             | 4.729(2)  | 4.818(2)  | 4.821(2)  |

TABLE V. Lattice constant, bulk modulus and atomization energy of Si calculated with a 3x3x3 *k-point* grid for various OPTM-GTO basis sets. Results with and without basis set corrections are presented.
